# Supplementary material for: Zero-Shot On-the-Fly Event Schema Induction
Source: arXiv:2210.06254 source file (2023-03-27)
Supplement: Supplementary file 1 [file Appendix_model_hyperparameters.tex]

\section{Model Implementation Details}
